# Supplementary material for: Color Shift Estimation-and-Correction for Image Enhancement
Source: arXiv:2405.17725 source file (2024-05-29)
Supplement: Supplementary file 1 [file X_suppl.tex]

\clearpage

\setcounter{page}{1}

\maketitlesupplementary

\begin{center}
    \author{Yiyu Li\qquad Ke Xu\qquad Gerhard Petrus Hancke\qquad Rynson W.H. Lau \\
City University of Hong Kong\\
% Institution1 address\\
{\tt\small \email{yiyuli.cs@my.cityu.edu.hk}, \email{kkangwing@gmail.com}, \{gp.hancke,  rynson.lau\}@cityu.edu.hk}
}
\end{center}

This supplementary material provides implementation details and more visual comparisons between the proposed method and seven state-of-the-art image enhancement methods, \ie, RetinexNet~\cite{wei_2018_BMVC_retinexnet}, MSEC~\cite{Afifi_2021_CVPR_MSEC}, SNRNet~\cite{Xu_2022_CVPR_SNR}, LCDP~\cite{Wang_2022_ECCV_lcdp}, RetinexFormer~\cite{cai_2023_retinexformer}, LANet~\cite{yang_2023_lanet}, and FECNet~\cite{Huang_2022_ECCV_Fourier}, in Figure~\ref{fig:visual-comparison1} and Figure~\ref{fig:visual-comparison2}.

\noindent \textbf{Implementation Details.}\quad We implement our model using PyTorch~\cite{paszke_2017_pytorch}. All our experiments are conducted on a single NVIDIA V100 GPU. The network parameters are optimized using Adam optimizer~\cite{kinga_2015_adam_optimizer} with $\beta_1 = 0.9$ and $\beta_2 = 0.999$. The learning rate is set to $1e^{-4}$. During training, we resize the image to $512\times 512$ and set the batch size to $6$. We implement our pseudo-normal feature generator with the same structure as our color shift modulation module and share their weights. For the loss functions, we empirically set the balancing hyper-parameters in Eq.~\ref{eq:loss1} and Eq.~\ref{eq:loss2} to $\lambda_1  = 1.0$, $\lambda_2 = 0.5$, $\lambda_3 = 1.0$, $\lambda_4 = 0.01$, $\lambda_p = 0.5$, and $\lambda_o = 1.0$. \yycr{The UNet-based feature extractor is the same as LCDPNet~\cite{Wang_2022_ECCV_lcdp}, which is a UNet with histogram information in different scales. The number of output channels of the $1\times 1$ convolution layers in COMO block is set to 16.}

\noindent \textbf{More Results.}\quad We can see that methods proposed for handling either over- or under-exposures (\ie, MSEC~\cite{Afifi_2021_CVPR_MSEC}, LANet~\cite{yang_2023_lanet}, and FECNet~\cite{Huang_2022_ECCV_Fourier}) cannot rectify the brightness of over- and under-exposed regions at the same time. For example, they either fail to restore the greenish color of under-exposed trees and grasses, or fail to restore the bluish color of the over-exposed sky (see Figure~\ref{fig:visual-comparison1} and Figure~\ref{fig:visual-comparison2} (c, g, and h)).
Methods originally proposed for low-light image enhancement (\ie, RetinexNet~\cite{wei_2018_BMVC_retinexnet}, SNRNet~\cite{Xu_2022_CVPR_SNR}, and RetinexFormer~\cite{cai_2023_retinexformer}) tend to increase the overall image brightness, which further buries the details of clouds (Figure~\ref{fig:visual-comparison1} and Figure~\ref{fig:visual-comparison2} (b, d, and f)).
LCDP~\cite{Wang_2022_ECCV_lcdp} is designed to deal with the coexistence of over- and under-exposure; however, the sky regions after the enhancement tend to have purplish colors (Figure~\ref{fig:visual-comparison1} and Figure~\ref{fig:visual-comparison2} (e)).
Similar problems can be found in the other case. In contrast, our method can enhance these images with better details and colors (Figure~\ref{fig:visual-comparison1} and Figure~\ref{fig:visual-comparison2} (i, s, and C)).

Figure~\ref{fig:real-world1} further shows our visual results of real-world images from the Flickr 30K~\cite{flickr30k} dataset. While existing methods tend to produce obvious color artifacts after their enhancements, our method can produce results of better visual quality.

\begin{figure*}[h]

\begin{center}

\begin{tabular}{ccccc}

    \includegraphics[width=0.19\linewidth]{comparison/a4105-07-11-26-at-16h02m57s-_MG_7151-lcdp.png} &
    \includegraphics[width=0.19\linewidth]{comparison/a4105-07-11-26-at-16h02m57s-_MG_7151-retinex.png} &
    \includegraphics[width=0.19\linewidth]{comparison/a4105-07-11-26-at-16h02m57s-_MG_7151-msec.png} &
    \includegraphics[width=0.19\linewidth]{comparison/a4105-07-11-26-at-16h02m57s-_MG_7151-snr.png} &
    \includegraphics[width=0.19\linewidth]{comparison/a4105-07-11-26-at-16h02m57s-_MG_7151-lcdp.png}\\ 
    \scriptsize{(a) Input} & \scriptsize{(b) RetinexNet~\cite{wei_2018_BMVC_retinexnet}}
    &\scriptsize{(c) MSEC~\cite{Afifi_2021_CVPR_MSEC}} & \scriptsize{(d) SNRNet~\cite{Xu_2022_CVPR_SNR}} & \scriptsize{(e) LCDP~\cite{Wang_2022_ECCV_lcdp}}\\

    \includegraphics[width=0.19\linewidth]{comparison/a4105-07-11-26-at-16h02m57s-_MG_7151-retinexformer.png} &
    \includegraphics[width=0.19\linewidth]{comparison/a4105-07-11-26-at-16h02m57s-_MG_7151-lanet.png} &
    \includegraphics[width=0.19\linewidth]{comparison/a4105-07-11-26-at-16h02m57s-_MG_7151-fec.png} &
    \includegraphics[width=0.19\linewidth]{comparison/a4105-07-11-26-at-16h02m57s-_MG_7151-ours.png} &
    \includegraphics[width=0.19\linewidth]{comparison/a4105-07-11-26-at-16h02m57s-_MG_7151-gt.png}\\ 
    \scriptsize{(f) RetinexFormer~\cite{cai_2023_retinexformer}} & \scriptsize{(g) LANet~\cite{yang_2023_lanet}}
    &\scriptsize{(h) FECNet~\cite{Huang_2022_ECCV_Fourier}} & \scriptsize{(i) Ours} & \scriptsize{(j) GT}\\

    % \includegraphics[width=0.19\linewidth]{comparison/a2995-dvf_068-input.png} &
    % \includegraphics[width=0.19\linewidth]{comparison/a2995-dvf_068-retinex.png} &
    % \includegraphics[width=0.19\linewidth]{comparison/a2995-dvf_068-msec.png} &
    % \includegraphics[width=0.19\linewidth]{comparison/a2995-dvf_068-snr.png} &
    % \includegraphics[width=0.19\linewidth]{comparison/a2995-dvf_068-lcdp.png}\\ 
    % \scriptsize{(u) Input} & \scriptsize{(v) RetinexNet~\cite{wei_2018_BMVC_retinexnet}}
    % &\scriptsize{(w) MSEC~\cite{Afifi_2021_CVPR_MSEC}} & \scriptsize{(x) SNRNet~\cite{Xu_2022_CVPR_SNR}} & \scriptsize{(y) LCDP~\cite{Wang_2022_ECCV_lcdp}}\\

    % \includegraphics[width=0.19\linewidth]{comparison/a2995-dvf_068-retinexformer.png} &
    % \includegraphics[width=0.19\linewidth]{comparison/a2995-dvf_068-lanet.png} &
    % \includegraphics[width=0.19\linewidth]{comparison/a2995-dvf_068-fec.png} &
    % \includegraphics[width=0.19\linewidth]{comparison/a2995-dvf_068-ours.png} &
    % \includegraphics[width=0.19\linewidth]{comparison/a2995-dvf_068-gt.png}\\ 
    % \scriptsize{(z) RetinexFormer~\cite{cai_2023_retinexformer}} & \scriptsize{(A) LANet~\cite{yang_2023_lanet}}
    % &\scriptsize{(B) FECNet~\cite{Huang_2022_ECCV_Fourier}} & \scriptsize{(C) Ours} & \scriptsize{(D) GT}\\

    \includegraphics[width=0.19\linewidth]{comparison/a2620-IMG_0099-input.png} &
    \includegraphics[width=0.19\linewidth]{comparison/a2620-IMG_0099-retinex.png} &
    \includegraphics[width=0.19\linewidth]{comparison/a2620-IMG_0099-msec.png} &
    \includegraphics[width=0.19\linewidth]{comparison/a2620-IMG_0099-snr.png} &
    \includegraphics[width=0.19\linewidth]{comparison/a2620-IMG_0099-lcdp.png}\\ 
    \scriptsize{(k) Input} & \scriptsize{(l) RetinexNet~\cite{wei_2018_BMVC_retinexnet}}
    &\scriptsize{(m) MSEC~\cite{Afifi_2021_CVPR_MSEC}} & \scriptsize{(n) SNRNet~\cite{Xu_2022_CVPR_SNR}} & \scriptsize{(o) LCDP~\cite{Wang_2022_ECCV_lcdp}}\\

    \includegraphics[width=0.19\linewidth]{comparison/a2620-IMG_0099-input.png} &
    \includegraphics[width=0.19\linewidth]{comparison/a2620-IMG_0099-lanet.png} &
    \includegraphics[width=0.19\linewidth]{comparison/a2620-IMG_0099-fec.png} &
    \includegraphics[width=0.19\linewidth]{comparison/a2620-IMG_0099-ours.png} &
    \includegraphics[width=0.19\linewidth]{comparison/a2620-IMG_0099-gt.png}\\ 
    \scriptsize{(p) RetinexFormer~\cite{cai_2023_retinexformer}} & \scriptsize{(q) LANet~\cite{yang_2023_lanet}}
    &\scriptsize{(r) FECNet~\cite{Huang_2022_ECCV_Fourier}} & \scriptsize{(s) Ours} & \scriptsize{(t) GT}\\

    \includegraphics[width=0.19\linewidth]{comparison/a1063-WP_CRW_4982-input.png} &
    \includegraphics[width=0.19\linewidth]{comparison/a1063-WP_CRW_4982-retinex.png} &
    \includegraphics[width=0.19\linewidth]{comparison/a1063-WP_CRW_4982-msec.png} &
    \includegraphics[width=0.19\linewidth]{comparison/a1063-WP_CRW_4982-snr.png} &
    \includegraphics[width=0.19\linewidth]{comparison/a1063-WP_CRW_4982-lcdp.png}\\ 
    \scriptsize{(u) Input} & \scriptsize{(v) RetinexNet~\cite{wei_2018_BMVC_retinexnet}}
    &\scriptsize{(w) MSEC~\cite{Afifi_2021_CVPR_MSEC}} & \scriptsize{(x) SNRNet~\cite{Xu_2022_CVPR_SNR}} & \scriptsize{(y) LCDP~\cite{Wang_2022_ECCV_lcdp}}\\

    \includegraphics[width=0.19\linewidth]{comparison/a1063-WP_CRW_4982-retinexformer.png} &
    \includegraphics[width=0.19\linewidth]{comparison/a1063-WP_CRW_4982-lanet.png} &
    \includegraphics[width=0.19\linewidth]{comparison/a1063-WP_CRW_4982-fec.png} &
    \includegraphics[width=0.19\linewidth]{comparison/a1063-WP_CRW_4982-ours.png} &
    \includegraphics[width=0.19\linewidth]{comparison/a1063-WP_CRW_4982-gt.png}\\ 
    \scriptsize{(z) RetinexFormer~\cite{cai_2023_retinexformer}} & \scriptsize{(A) LANet~\cite{yang_2023_lanet}}
    &\scriptsize{(B) FECNet~\cite{Huang_2022_ECCV_Fourier}} & \scriptsize{(C) Ours} & \scriptsize{(D) GT}\\
    
\end{tabular}
\end{center}
\vspace{-5mm}
\caption{Visual comparison between our method and state-of-the-art methods on LCDP~\cite{Wang_2022_ECCV_lcdp} dataset, which has images with both over-exposure and under-exposure.}
\vspace{-5mm}
\label{fig:visual-comparison1}
\end{figure*}

\vspace{-3mm}
\begin{figure*}[h!]

\begin{center}

\begin{tabular}{ccccc}

    \includegraphics[width=0.19\linewidth]{comparison/a4044-IMG_1634-input.png} &
    \includegraphics[width=0.19\linewidth]{comparison/a4044-IMG_1634-retinex.png} &
    \includegraphics[width=0.19\linewidth]{comparison/a4044-IMG_1634-msec.png} &
    \includegraphics[width=0.19\linewidth]{comparison/a4044-IMG_1634-snr.png} &
    \includegraphics[width=0.19\linewidth]{comparison/a4044-IMG_1634-lcdp.png}\\ 
    \scriptsize{(a) Input} & \scriptsize{(b) RetinexNet~\cite{wei_2018_BMVC_retinexnet}}
    &\scriptsize{(c) MSEC~\cite{Afifi_2021_CVPR_MSEC}} & \scriptsize{(d) SNRNet~\cite{Xu_2022_CVPR_SNR}} & \scriptsize{(e) LCDP~\cite{Wang_2022_ECCV_lcdp}}\\

    \includegraphics[width=0.19\linewidth]{comparison/a4044-IMG_1634-retinexformer.png} &
    \includegraphics[width=0.19\linewidth]{comparison/a4044-IMG_1634-lanet.png} &
    \includegraphics[width=0.19\linewidth]{comparison/a4044-IMG_1634-fec.png} &
    \includegraphics[width=0.19\linewidth]{comparison/a4044-IMG_1634-ours.png} &
    \includegraphics[width=0.19\linewidth]{comparison/a4044-IMG_1634-gt.png}\\ 
    \scriptsize{(f) RetinexFormer~\cite{cai_2023_retinexformer}} & \scriptsize{(g) LANet~\cite{yang_2023_lanet}}
    &\scriptsize{(h) FECNet~\cite{Huang_2022_ECCV_Fourier}} & \scriptsize{(i) Ours} & \scriptsize{(j) GT}\\

    \includegraphics[width=0.19\linewidth]{comparison/a1940-jmac_MG_6206-input.png} &
    \includegraphics[width=0.19\linewidth]{comparison/a1940-jmac_MG_6206-retinex.png} &
    \includegraphics[width=0.19\linewidth]{comparison/a1940-jmac_MG_6206-msec.png} &
    \includegraphics[width=0.19\linewidth]{comparison/a1940-jmac_MG_6206-snr.png} &
    \includegraphics[width=0.19\linewidth]{comparison/a1940-jmac_MG_6206-lcdp.png}\\ 
    \scriptsize{(k) Input} & \scriptsize{(l) RetinexNet~\cite{wei_2018_BMVC_retinexnet}}
    &\scriptsize{(m) MSEC~\cite{Afifi_2021_CVPR_MSEC}} & \scriptsize{(n) SNRNet~\cite{Xu_2022_CVPR_SNR}} & \scriptsize{(o) LCDP~\cite{Wang_2022_ECCV_lcdp}}\\

    \includegraphics[width=0.19\linewidth]{comparison/a1940-jmac_MG_6206-retinexformer.png} &
    \includegraphics[width=0.19\linewidth]{comparison/a1940-jmac_MG_6206-lanet.png} &
    \includegraphics[width=0.19\linewidth]{comparison/a1940-jmac_MG_6206-fec.png} &
    \includegraphics[width=0.19\linewidth]{comparison/a1940-jmac_MG_6206-ours.png} &
    \includegraphics[width=0.19\linewidth]{comparison/a1940-jmac_MG_6206-gt.png}\\ 
    \scriptsize{(p) RetinexFormer~\cite{cai_2023_retinexformer}} & \scriptsize{(q) LANet~\cite{yang_2023_lanet}}
    &\scriptsize{(r) FECNet~\cite{Huang_2022_ECCV_Fourier}} & \scriptsize{(s) Ours} & \scriptsize{(t) GT}\\

    \includegraphics[width=0.19\linewidth]{comparison/a2995-dvf_068-input.png} &
    \includegraphics[width=0.19\linewidth]{comparison/a2995-dvf_068-retinex.png} &
    \includegraphics[width=0.19\linewidth]{comparison/a2995-dvf_068-msec.png} &
    \includegraphics[width=0.19\linewidth]{comparison/a2995-dvf_068-snr.png} &
    \includegraphics[width=0.19\linewidth]{comparison/a2995-dvf_068-lcdp.png}\\ 
    \scriptsize{(u) Input} & \scriptsize{(v) RetinexNet~\cite{wei_2018_BMVC_retinexnet}}
    &\scriptsize{(w) MSEC~\cite{Afifi_2021_CVPR_MSEC}} & \scriptsize{(x) SNRNet~\cite{Xu_2022_CVPR_SNR}} & \scriptsize{(y) LCDP~\cite{Wang_2022_ECCV_lcdp}}\\

    \includegraphics[width=0.19\linewidth]{comparison/a2995-dvf_068-retinexformer.png} &
    \includegraphics[width=0.19\linewidth]{comparison/a2995-dvf_068-lanet.png} &
    \includegraphics[width=0.19\linewidth]{comparison/a2995-dvf_068-fec.png} &
    \includegraphics[width=0.19\linewidth]{comparison/a2995-dvf_068-ours.png} &
    \includegraphics[width=0.19\linewidth]{comparison/a2995-dvf_068-gt.png}\\ 
    \scriptsize{(z) RetinexFormer~\cite{cai_2023_retinexformer}} & \scriptsize{(A) LANet~\cite{yang_2023_lanet}}
    &\scriptsize{(B) FECNet~\cite{Huang_2022_ECCV_Fourier}} & \scriptsize{(C) Ours} & \scriptsize{(D) GT}\\
    
\end{tabular}
\end{center}
\vspace{-5mm}
\caption{Visual comparison between our method and state-of-the-art methods on LCDP~\cite{Wang_2022_ECCV_lcdp} dataset, which has images with both over-exposure and under-exposure.}
% \vspace{-5mm}
\label{fig:visual-comparison2}
\end{figure*}

\begin{figure}[h]

\begin{center}

\begin{tabular}{cccc}

    \includegraphics[width=0.24\linewidth]{real-world-examples/898-input.png} &
    \includegraphics[width=0.24\linewidth]{real-world-examples/898-msec.png} &
    \includegraphics[width=0.24\linewidth]{real-world-examples/898-lcdp.png} &
    \includegraphics[width=0.24\linewidth]{real-world-examples/898-ours.png}\\

    \includegraphics[width=0.24\linewidth]{real-world-examples/336-input.png} &
    \includegraphics[width=0.24\linewidth]{real-world-examples/336-msec.png} &
    \includegraphics[width=0.24\linewidth]{real-world-examples/336-lcdp.png} &
    \includegraphics[width=0.24\linewidth]{real-world-examples/336-ours.png}\\

    \includegraphics[width=0.24\linewidth]{real-world-examples/7768-input.png} &
    \includegraphics[width=0.24\linewidth]{real-world-examples/7768-msec.png} &
    \includegraphics[width=0.24\linewidth]{real-world-examples/7768-lcdp.png} &
    \includegraphics[width=0.24\linewidth]{real-world-examples/7768-ours.png}\\

    \includegraphics[width=0.24\linewidth]{real-world-examples/9384-input.png} &
    \includegraphics[width=0.24\linewidth]{real-world-examples/9384-msec.png} &
    \includegraphics[width=0.24\linewidth]{real-world-examples/9384-lcdp.png} &
    \includegraphics[width=0.24\linewidth]{real-world-examples/9384-ours.png}\\

    \includegraphics[width=0.24\linewidth]{real-world-examples/5871970-input.png} &
    \includegraphics[width=0.24\linewidth]{real-world-examples/5871970-msec.png} &
    \includegraphics[width=0.24\linewidth]{real-world-examples/5871970-lcdp.png} &
    \includegraphics[width=0.24\linewidth]{real-world-examples/5871970-ours.png}\\
    
    \scriptsize{Input} & \scriptsize{MSEC~\cite{Afifi_2021_CVPR_MSEC}}
    &\scriptsize{LCDP~\cite{Wang_2022_ECCV_lcdp}} & \scriptsize{Ours}\\
    
\end{tabular}
\end{center}
\vspace{-5mm}
\caption{Visual results of real-world examples from the Flickr 30K~\cite{flickr30k} dataset. Our method produces better visual results.}
\vspace{-5mm}
\label{fig:real-world1}
\end{figure}
